# Supplementary material for: Same Stories, Different Journeys: Exploring Persona-Grounded Conversational Agents for Supporting Career Exploration with Peers' Posts
Source: arXiv:2607.11039 source file (2026-09-23)
Supplement: Supplementary file 1 [file appendix.tex]

%%
%% UIST 2026 Submission: JobMate — Supplementary Materials (separate PDF)
%%
\documentclass[sigconf]{acmart}

\AtBeginDocument{%
  }

\usepackage{booktabs}
\usepackage{graphicx}
\usepackage{balance}
\usepackage{xcolor}
\usepackage{soul}
\usepackage{listings}
\usepackage{enumitem}

\lstset{
  basicstyle=\ttfamily\footnotesize,
  breaklines=true,
  breakatwhitespace=true,
  frame=single,
  framesep=4pt,
  xleftmargin=1em,
  xrightmargin=1em,
  showstringspaces=false,
  tabsize=2,
  columns=fullflexible,
  keepspaces=true
}

\setcopyright{none}
\settopmatter{printacmref=false}
\acmConference[Preprint]{Preprint}{2026}{}
\acmYear{2026}
\copyrightyear{2026}
\acmDOI{}
\acmISBN{}

\begin{document}

\title{Supplementary Materials}

\maketitle

%% ============================================================
%% A. FORMATIVE STUDY — INTERVIEWERS AND INTERVIEW PARTICIPANTS
%% ============================================================
\section{Formative Study Participants}
\label{sec:supp-formative}

We conducted semi-structured formative interviews with $N{=}8$ participants who were navigating career decisions and reported using social media for job-related information (e.g., interview tips, compensation signals, and employer or role discovery). The sessions elicited practices, friction points, and design directions that informed JobMate; thematic findings appear in the main paper. Table~\ref{tab:formative-participants} summarizes self-reported program background, degree stage, gender, and age. Institution names are omitted for anonymized review.

\begin{table*}[t]
  \caption{Formative interview participants ($N{=}8$): self-reported program/discipline, degree stage, gender, and age.}
  \label{tab:formative-participants}
  \centering
  \small
  \setlength{\tabcolsep}{4pt}
  \begin{tabular}{@{}c p{0.62\textwidth} l c c@{}}
    \toprule
    ID & Program / discipline (summary) & Degree stage & Sex & Age \\
    \midrule
    P1 & Law (undergraduate and master's) & Master's, final yr. & F & 24 \\
    P2 & Life sciences; bioinformatics (doctoral) & Doctoral, Yr.~2 & F & 28 \\
    P3 & Telecommunications / electrical engineering (master's) & Master's, final yr. & M & 25 \\
    P4 & Pharmacy (undergraduate) & Undergraduate, final yr. & F & 22 \\
    P5 & Chemistry (master's) & Master's, final yr. & M & 25 \\
    P6 & Mathematics (undergraduate) & Undergraduate, final yr. & F & 22 \\
    P7 & Computer science (master's) & Master's, Yr.~2 & F & 24 \\
    P8 & Traditional Chinese medicine (master's) & Master's, Yr.~1 & F & 24 \\
    \bottomrule
  \end{tabular}
\end{table*}

%% ============================================================
%% B. USER STUDY PARTICIPANTS
%% ============================================================
\section{User Study Participants}
\label{sec:supp-user-study}

We conducted a between-subjects lab study with $N{=}24$ participants comparing JobMate with native RedNote browsing. Participants were stratified by self-reported major into three discipline groups---computer science, psychology, and Chinese literature---with eight participants per discipline. Within each discipline, four participants were assigned to JobMate and four to RedNote, yielding 12 participants per condition overall. Table~\ref{tab:user-study-participants} lists anonymized identifiers alongside self-reported discipline, age, gender, and condition. Names, session dates/times, recruitment handles, and network identifiers are withheld for anonymized review.

\begin{table*}[t]
  \caption{User study participants ($N{=}24$): self-reported discipline, age, gender, and between-subjects condition (JobMate vs.\ native RedNote). IDs are arbitrary row order from recruitment logs.}
  \label{tab:user-study-participants}
  \centering
  \footnotesize
  \setlength{\tabcolsep}{3.5pt}
  \begin{tabular}{@{}c l c c l@{}}
    \toprule
    ID & Discipline & Age & Sex & Condition \\
    \midrule
    P1  & Computer science      & 25 & F & JobMate \\
    P2  & Psychology            & 22 & F & JobMate \\
    P3  & Psychology            & 19 & F & JobMate \\
    P4  & Psychology            & 24 & F & RedNote \\
    P5  & Computer science      & 24 & F & JobMate \\
    P6  & Psychology            & 19 & F & RedNote \\
    P7  & Psychology            & 19 & F & JobMate \\
    P8  & Psychology            & 19 & F & RedNote \\
    P9  & Chinese literature    & 23 & F & JobMate \\
    P10 & Chinese literature    & 21 & F & RedNote \\
    P11 & Psychology            & 22 & M & JobMate \\
    P12 & Chinese literature    & 23 & F & RedNote \\
    P13 & Psychology            & 18 & M & RedNote \\
    P14 & Chinese literature    & 18 & F & JobMate \\
    P15 & Chinese literature    & 22 & F & RedNote \\
    P16 & Computer science      & 19 & M & RedNote \\
    P17 & Computer science      & 19 & M & RedNote \\
    P18 & Computer science      & 19 & M & RedNote \\
    P19 & Computer science      & 19 & M & RedNote \\
    P20 & Computer science      & 21 & M & JobMate \\
    P21 & Computer science      & 24 & F & JobMate \\
    P22 & Chinese literature    & 21 & F & RedNote \\
    P23 & Chinese literature    & 24 & F & JobMate \\
    P24 & Chinese literature    & 20 & F & JobMate \\
    \bottomrule
  \end{tabular}
\end{table*}

%% ============================================================
%% C. QUESTIONNAIRES AND MEASURES
%% ============================================================
\section{Questionnaires and Measures}
\label{sec:supp-questionnaires}

The user study battery comprised (i)~34 career-decision difficulty items, (ii)~six NASA--TLX-style workload dimensions, (iii)~nine study-specific items on support and system experience, and (iv)~12 self-determination--style items on career decision-making, in the order listed below (same order as the deployed Chinese questionnaire in our study materials).
Pre- versus post-task administration and any condition-specific wording branches follow the procedure described in the main paper.
\input{appendix_questionnaires}

%% ============================================================
%% D. LLM PROMPTS — DATA PROCESSING
%% ============================================================
\section{LLM Prompts for Data Processing}
\label{sec:supp-data-prompts}

The ingestion pipeline uses two LLM steps: (1)~\texttt{classify\_post}---validity screening and post-type labeling---and (2)~\texttt{extract\_detailed\_persona}---structured persona fields (background, outcome, tags, struggle summary) from post title and body.
Listings~\ref{lst:prompt-data-classify} and~\ref{lst:prompt-data-persona} give \textbf{English translations} of the deployed system prompts (production text was Chinese; see repository file \texttt{all\_material/prompt.txt}).

\input{appendix_prompts_data_english}

%% ============================================================
%% E. LLM PROMPTS — CONVERSATION
%% ============================================================
\section{LLM Prompts for Conversational Agent}
\label{sec:supp-chat-prompts}

The conversational stack uses \texttt{generateGreeting} for the opening turn, with a fixed user message asking the model to greet the participant and suggest three starter questions or topics (Chinese in deployment; functionally equivalent to the English gloss in Listing~\ref{lst:prompt-chat-greeting}).
\texttt{buildChatSystemPrompt} supplies the multi-turn system message.
Template literals (e.g., \texttt{\$\{agent.background\_info\}}, \texttt{\$\{relatedPostsText\}}) inject persona fields, onboarding answers, and retrieved related-post text at runtime.
Listings~\ref{lst:prompt-chat-greeting}--\ref{lst:prompt-api} summarize prompts and default API settings (\texttt{gpt-4o-mini}, sampling parameters).

\input{appendix_prompts_chat_english}

\begin{acks}
[Anonymized for review.]
\end{acks}

\end{document}
